# Supplementary material for: Managing the Uncertainty in System Dynamics Through Distributionally Robust Stability-Constrained Optimization
Source: arXiv:2309.03798 source file (2024-04-22)
Supplement: Supplementary file 2 [file SM.tex]

%%%%%%%%%%%%%%%%%%%%%%%%%%%%%%%%%%%%%%%%
% Damping SI ^ 2
%%%%%%%%%%%%%%%%%%%%%%%%%%%%%%%%%%%%%%%%

\documentclass[tightpage]{standalone}

% import style library
\usepackage{myStyleIEEE}

\begin{document}

\begin{varwidth}{\linewidth}

\begin{tikzpicture}
\begin{axis}[
    scaled ticks=false,
    tick label style={/pgf/number format/fixed},
    colormap name=viridis,
    width=7.25cm,
    height=4cm,
    %trim axis left,
    %trim axis right,
    %xlabel style={yshift=0.75em},
    %ylabel style={yshift=-1.5em},
    xlabel={$\mathrm{Stiblity\, Margin\,[\%]}$},
    ylabel={\ref{pgfplots:Cost} $\mathrm{Cost\,[k\pounds/h]}$},
    xmin=0, xmax=20,
    ymin=280, ymax=370,
    % ytick={280,296,312,328,344,360},
    % yticklabel style={/pgf/number format/.cd,fixed,precision=3},
    %legend pos=north east,
    xmajorgrids=true,
    ymajorgrids=true,
    legend cell align={left},
    grid style=dashed,
]
\footnotesize
\addplot[
    % smooth,
    % dashed,
    thick,
    color=pBlue,
    %fill=black, 
    %fill opacity=0.15
    ]
    table {data/SM/data0.txt};  
    \label{pgfplots:Cost}
    % \addlegendentry{\footnotesize Base Case} 
\end{axis}
\begin{axis}[
    % scaled y ticks=base 10:1,
    tick label style={font=\footnotesize},
    label style={font=\footnotesize},
    colormap name=viridis,
    width=7.25cm,
    height=4cm,
    axis y line*=right,
    axis x line=none,
    %trim axis left,
    %trim axis right,
    %xlabel style={yshift=0.75em},
    %ylabel style={yshift=-1.5em},
    ylabel={\ref{pgfplots:Ds} $\mathrm{Violation \,Rate\,[\%]} $},
    xmin=0, xmax=20,
    ymin=0, ymax=9,
    ytick={0,2,4,6,8},
    % yticklabel style={/pgf/number format/.cd,fixed zerofill,precision=1},
    %legend pos=north east,
    % xmajorgrids=true,
    % ymajorgrids=true,
    % legend style={at={(axis cs:71.7,71)},anchor=north east,nodes={scale=0.7, transform shape},legend columns=3},
    % legend cell align={left},
    % grid style=dashed,
]
  
% \addlegendimage{/pgfplots/refstyle=plot_one}\addlegendentry{plot 1}
% \addlegendimage{/pgfplots/refstyle=plot_two}\addlegendentry{plot 2}

\addplot[
    % smooth,
    thick,
    color=pRed,
    %fill=black, 
    %fill opacity=0.15
    ]
    table {data/SM/data1.txt};  % \addlegendentry{\footnotesize $H_s$}  
    \label{pgfplots:Ds}
    
\end{axis}
\end{tikzpicture} 

\end{varwidth}
\end{document}
